# Supplementary material for: Nernst Plateau in the Quantum Limit of Low-Carrier-Density Topological Insulators
Source: arXiv:2409.07199 source file (2026-05-04)
Supplement: Supplementary file 1 [file NernstPlateau_SM240822.pdf]

# Supplemental Material for “Nernst Plateau in the Quantum Limit of Topological Insulators”

Peng-Lu Zhao,<sup>1,2</sup> J. L. Zhang,<sup>3,\*</sup> Hai-Zhou Lu,<sup>2,4,5,†</sup> and Qian Niu<sup>1,6</sup>

<sup>1</sup>*Department of Physics, University of Science and Technology of China, Hefei, Anhui 230026, China*

<sup>2</sup>*Department of Physics, Southern University of Science and Technology (SUSTech), Shenzhen 518055, China*

<sup>3</sup>*Anhui Key Laboratory of Condensed Matter Physics at Extreme Conditions,*

*High Magnetic Field Laboratory, HFIPS, Chinese Academy of Sciences, Hefei 230031, China*

<sup>4</sup>*Quantum Science Center of Guangdong-Hong Kong-Macao Greater Bay Area (Guangdong), Shenzhen 518045, China*

<sup>5</sup>*International Quantum Academy, Shenzhen 518048, China*

<sup>6</sup>*CAS Key Laboratory of Strongly-Coupled Quantum Matter Physics, University of Science and Technology of China, Hefei, Anhui 230026, China*

## CONTENTS

|                                                                      |    |
|----------------------------------------------------------------------|----|
| I. Model                                                             | 1  |
| II. Landau bands                                                     | 2  |
| III. Critical magnetic fields for Weyl points formation.             | 3  |
| IV. Calculations of conductivities                                   | 4  |
| A. Longitudinal conductivity                                         | 5  |
| B. Hall conductivity                                                 | 5  |
| V. Fixing Carrier Density vs. Fixing Fermi Energy                    | 6  |
| VI. Value of the critical magnetic field for the Lifshitz transition | 7  |
| VII. Analytical value of the flat Nernst coefficient                 | 7  |
| A. Weak topological insulators                                       | 8  |
| B. Strong topological insulators                                     | 10 |
| VIII. Calculation of the the energy broadening parameter             | 11 |
| A. Weak topological insulators                                       | 12 |
| B. Strong topological insulators                                     | 12 |
| References                                                           | 14 |

## I. MODEL

3D strong and weak topological insulators can generally be characterized using an adapted Dirac model [1],

$$H_0(\mathbf{k}) = \hbar v_x k_x \tau_z \sigma_x + \hbar v_y k_y \tau_0 \sigma_y + \hbar v_z k_z \tau_x \sigma_x + [\Delta + M_\perp (k_x^2 + k_y^2) + M_z k_z^2] \tau_0 \sigma_z. \quad (1)$$

This model describes a 3D Dirac semimetal if  $\Delta = 0$ ; otherwise, it could describe a normal insulators, a weak topological insulator, or a strong topological insulator, depending on the relative sign of the bulk gap  $\Delta$  and band inversion parameters  $M_\perp$ ,  $M_z$ . Here, we consider the insulating case with  $\Delta \neq 0$ . To distinguish the topological nature, we define four  $Z_2$  indices ( $\nu_0; \nu_{j=1-3}$ ) according to [2, 3],

$$(-1)^{\nu_0} = \prod_i \prod_{n=1}^{N/2} \xi_n(\Gamma_i) \quad (2)$$

---

\* zhangjinglei@hmfl.ac.cn

† luhz@sustech.edu.cn

where  $\xi_n(\Gamma_i) = \pm 1$  are the eigenvalues of inversion symmetry  $\mathcal{I} = \tau_0 \sigma_z$  for the  $n$ -th occupied energy band at eight time-reversal invariant  $k$ -points:

$$\Gamma_i \in \{(0, 0, 0), (\pi, \pi, 0), (0, 0, \pi), (0, \pi, 0), (\pi, \pi, 0), (\pi, 0, \pi), (\pi, 0, 0), (\pi, 0, \pi)\}. \quad (3)$$

$\nu_{j=1-3}$  are defined similarly but with four  $k$ -points having  $k_j = \pi$ . To determine the weak or strong TI, we use the continuum model for Eq. (1),

$$H(\mathbf{k}) = A \sin(k_x a) \tau_z \sigma_x + B \sin(k_y a) \tau_0 \sigma_y + C \sin(k_z a) \tau_x \sigma_x \\ + \left\{ \Delta + D \left[ \sin^2 \left( \frac{k_x a}{2} \right) + \sin^2 \left( \frac{k_y a}{2} \right) \right] + F \sin^2 \left( \frac{k_z a}{2} \right) \right\} \tau_0 \sigma_z. \quad (4)$$

The band parameters are given by

$$Aa = \hbar v_x, \quad Ba = -\hbar v_y k_y, \quad Ca = \hbar v_z, \quad \frac{Da^2}{4} = M, \quad \frac{Fa^2}{4} = M_z, \quad (5)$$

We used  $a$  as the general lattice constant although the anisotropy permits three lattice constants. This simplification will not affect our conclusions. Based on Eq. (4), the four  $Z_2$  indices are obtained,

$$(-1)^{\nu_0} = \text{sgn} [\Delta (\Delta + F) (\Delta + 2D) (\Delta + 2D + F)]; \\ (-1)^{\nu_1} = (-1)^{\nu_2} = \text{sgn} [(\Delta + D) (\Delta + D + F) (\Delta + 2D) (\Delta + 2D + F)]; \\ (-1)^{\nu_3} = \text{sgn} [(\Delta + F) (\Delta + D + F)^2 (\Delta + 2D + F)]. \quad (6)$$

Without loss of generality, we fix  $\Delta > 0$ , leading to four cases in Eq. (6):

$$\begin{aligned} \text{(I)} \quad D > 0, F > 0 &\Leftrightarrow M > 0, M_z > 0; \quad (\nu_0; \nu_j) = (0, 000) \Rightarrow \text{Normal insulator} \\ \text{(II)} \quad D < 0, F > 0 &\Leftrightarrow M < 0, M_z > 0; \quad (\nu_0; \nu_j) = (0, 001) \Rightarrow \text{Weak TI} \\ \text{(III)} \quad F < D < 0 &\Leftrightarrow M_z < M < 0; \quad (\nu_0; \nu_j) = (1, 001) \Rightarrow \text{Strong TI} \\ \text{(IV)} \quad D < F < 0 &\Leftrightarrow M < M_z < 0; \quad (\nu_0; \nu_j) = (0, 001) \Rightarrow \text{Weak TI.} \end{aligned} \quad (7)$$

These four cases are consistent with the results obtained from previous DFT calculations [4].

## II. LANDAU BANDS

Applying a magnetic fields along the  $z$ -direction,  $\mathbf{B} = (0, 0, B)$ , the canonical momentum are obtained by the Peierls substitution  $\mathbf{\Pi} = \mathbf{k} + e\mathbf{A}/\hbar$  with  $\mathbf{A} = (-yB, 0, 0)$ . As a result,  $k_x$  and  $k_z$  are still good quantum numbers. The ladder operators are defined by,

$$a = \frac{\ell_B}{\sqrt{2}\hbar v_\perp} (\hbar v_x \Pi_x - i\hbar v_y \Pi_y), \quad a^\dagger = \frac{\ell_B}{\sqrt{2}\hbar v_\perp} (\hbar v_x \Pi_x + i\hbar v_y \Pi_y). \quad (8)$$

where  $v_\perp = \sqrt{v_x v_y}$ , and the magnetic length is  $\ell_B = \sqrt{\frac{\hbar}{eB}}$ . Then, the Hamiltonian Eq. (1) can be written as

$$H_0 = \begin{bmatrix} M(\hat{n}, k_z) & \frac{\sqrt{2}}{\ell_B} \hbar v_\perp a^\dagger & 0 & \hbar v_z k_z \\ \frac{\sqrt{2}}{\ell_B} \hbar v_\perp a & -M(\hat{n}, k_z) & \hbar v_z k_z & 0 \\ 0 & \hbar v_z k_z & M(\hat{n}, k_z) & -\frac{\sqrt{2}}{\ell_B} \hbar v_\perp a \\ \hbar v_z k_z & 0 & -\frac{\sqrt{2}}{\ell_B} \hbar v_\perp a^\dagger & -M(\hat{n}, k_z) \end{bmatrix} \quad (9)$$

where  $M(\hat{n}, k_z) = \Delta + \frac{2M_\perp}{\ell_B^2} (\hat{n} + \frac{1}{2}) + M_z k_z^2$ , and  $M_\perp$  is defined by the axial approximation [5, 6],

$$\frac{M_x}{v_x^2} \approx \frac{M_y}{v_y^2} = \frac{M_\perp}{v_\perp^2}. \quad (10)$$

We further introduce the Zeeman term as [7, 8],

$$H_Z = -g \frac{\mu_B B}{2} \tau_z \sigma_0 = -Z \tau_z \sigma_0 \quad (11)$$

where  $g$  representing the Landé  $g$  factor, and  $\bar{Z} = g\mu_B B/2$  standing for the Zeeman energy. With Zeeman term, the eigenvalues of the total Hamiltonian for  $v_z = 0$  [8, 9] are given by

$$E_{n\nu}^\mu(k_z) = \mu (Z - M_\perp/\ell_B^2) + \nu \sqrt{(M_z k_z^2 + 2M_\perp n/\ell_B^2 + \Delta)^2 + (\sqrt{2n}\hbar v_\perp/\ell_B)^2}, \quad (12)$$

where  $n \geq 1$  representing the  $n$ -Landau level and  $\mu, \nu = \pm$ . The corresponding eigenvectors are

$$\begin{aligned} |n\mathbf{k}, +(\nu), +(\mu)\rangle &= \left[ 0, 0, -\cos \frac{\theta_n^+}{2} |n-1\rangle, \sin \frac{\theta_n^+}{2} |n\rangle \right]^T |k_x, k_z\rangle; \quad |n\mathbf{k}, -, +\rangle = \left[ 0, 0, \sin \frac{\theta_n^+}{2} |n-1\rangle, \cos \frac{\theta_n^+}{2} |n\rangle \right]^T |k_x, k_z\rangle \\ |n\mathbf{k}, +, -\rangle &= \left[ \cos \frac{\theta_n^-}{2} |n\rangle, \sin \frac{\theta_n^-}{2} |n-1\rangle, 0, 0 \right]^T |k_x, k_z\rangle; \quad |n\mathbf{k}, -, -\rangle = \left[ -\sin \frac{\theta_n^-}{2} |n\rangle, \cos \frac{\theta_n^-}{2} |n-1\rangle, 0, 0 \right]^T |k_x, k_z\rangle, \end{aligned} \quad (13)$$

where  $\cos \theta_n^\mu = \frac{M_z k_z^2 + 2M_\perp n/\ell_B^2 + \Delta}{\sqrt{(M_z k_z^2 + 2M_\perp n/\ell_B^2 + \Delta)^2 + (\sqrt{2n}\hbar v_\perp/\ell_B)^2}}$  and  $\theta_n^\mu \in (0, \pi)$ , and  $\{|n\rangle\}$  represent the eigenstates of the occupation number operator, which in real space read

$$\psi_{n,k_x,k_z}(\mathbf{r}) = \langle \mathbf{r} | n \rangle |k_x, k_z\rangle = \frac{C_n}{\sqrt{L_x L_z \ell_B}} e^{i(k_x x + k_z z)} e^{-\frac{(y-y_0)^2}{2\ell_B^2}} \mathcal{H}_n \left( \frac{y-y_0}{\ell_B} \right), \quad (14)$$

where  $C_n \equiv 1/\sqrt{n!2^n\sqrt{\pi}}$ ,  $L_x L_z$  is area of sample,  $y_0 = k_x \ell_B^2$  is the guiding center, and  $\mathcal{H}_n$  are the Hermite polynomials. We would like to remind you that each eigenvector above can also be multiplied by an overall phase factor, which does not affect anything. For  $n = 0$ , the eigenvalues take the form,

$$E_{0\nu}^\mu(k_z) = \nu \sqrt{(M_z k_z^2 + M_\perp/\ell_B^2 + \Delta - Z)^2 + (\hbar v_z k_z)^2}. \quad (15)$$

Here,  $E_{0\nu}^\mu(k_z)$  are independent on  $\mu = \pm$ , and are only two energy levels. To have a universal labels for all Landau levels, we keep such  $\pm$  in lowest Landau levels.

### III. CRITICAL MAGNETIC FIELDS FOR WEYL POINTS FORMATION.

To demonstrate the formation of Weyl points when the magnetic field is sufficiently strong, we employ the approximation  $v_z = 0$  taken in [8, 9], thus transforming Eq. (16) into

$$E_{0\nu}(k_z) = \nu |M_z k_z^2 + M_\perp/\ell_B^2 + \Delta - Z|. \quad (16)$$

As shown in Fig. 1(a), for small magnetic fields,  $M_z k_z^2 + M_\perp/\ell_B^2 + \Delta - Z > 0$  for any  $k_z$ , leading to  $E_{0\nu=+}(k_z)$  and  $E_{0\nu=-}(k_z)$  being distinct normal bands without intersection. When the magnetic field is sufficiently large (Fig. 1(b)),  $M_z k_z^2 + M_\perp/\ell_B^2 + \Delta - Z$  can become zero, resulting in the convergence of  $E_{0\nu=+}(k_z)$  and  $E_{0\nu=-}(k_z)$ , forming a pair of Weyl points at  $k_z = \pm k_w$ , the positions of Weyl points can therefore be obtained from the following equation

$$M_z k_w^2 + M_\perp/\ell_B^2 + \Delta - Z = 0, \quad (17)$$

which gives rise to a real  $k_w$  once  $(Z - M_\perp/\ell_B^2 - \Delta)/M_z \geq 0$ . For weak topological insulators,  $M_\perp < 0$  and  $M_z > 0$  [4, 8] a real  $k_w$  can be obtained for a sufficiently large  $B$ , and the critical value of  $B$  is

$$B_1 = \Delta / (-M_\perp e/\hbar + g\mu_B/2). \quad (18)$$

When  $B > B_1$ , Eq. (17) provides

$$k_z = k_w = \sqrt{\frac{Z - M_\perp/\ell_B^2 - \Delta}{M_z}} = \sqrt{\frac{(-M_\perp e/\hbar + g\mu_B/2) B - \Delta}{M_z}}, \quad (19)$$

which indicates that the position of the Weyl point increases with the magnetic field by  $\sqrt{B}$ .

In contrast to the behavior exhibited by the normal bands (Fig. 1(a)),  $E_{0\nu=+}(k_z)$  and  $E_{0\nu=-}(k_z)$  demonstrate band inversions within the range of  $k_z$  lying between the two Weyl points (Fig. 1(b)). Due to these band inversions, the eigenstates of  $E_{0\nu=\pm}(k_z)$  differ for  $|k_z| > k_w$  and  $|k_z| < k_w$ , leading to increased complexity in our subsequent calculations. To simplify, we use an alternative band labeling,

$$E_{0\xi}(k_z) = \xi (M_z k_z^2 + M_\perp / \ell_B^2 + \Delta - Z), \quad (20)$$

and the associated eigenstates are given by

$$|0, \xi = +\rangle = [|0\rangle, 0, 0, 0]^T |k_x, k_z\rangle; \quad |0, \xi = -\rangle = [0, 0, 0, |0\rangle]^T |k_x, k_z\rangle. \quad (21)$$

The two bands  $E_{0\xi=\pm}$  are plotted in Fig. 1(c). In the following calculations,  $E_{0\pm}$  denotes  $\xi = \pm$ , and the associated eigenvectors follow suit. We have confirmed that using  $E_{0\nu=\pm}$  and their corresponding eigenvectors produces the same results.

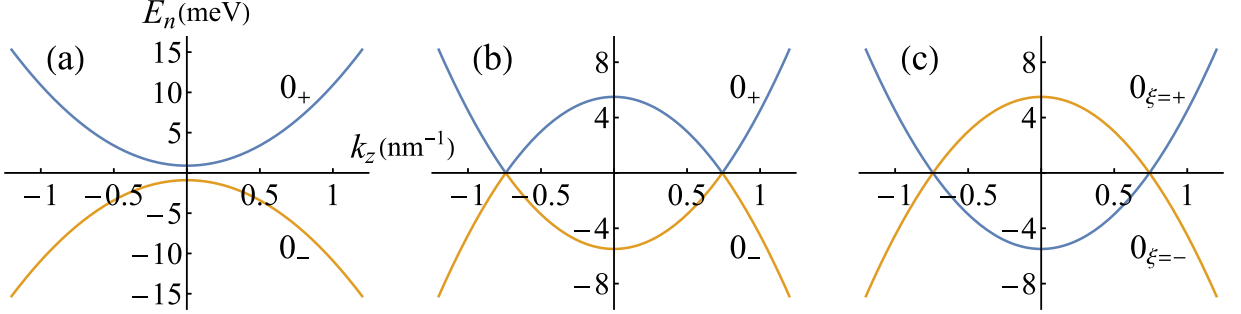

FIG. 1. (a), (b) The Lowest Landau bands plotted using Eq. (16) with  $M_z = 1 \text{ eV} \cdot \text{\AA}^2$ ,  $M_\perp = -12.24 \text{ eV} \cdot \text{\AA}^2$ ,  $g = 12$ ,  $\Delta = 2.5 \text{ meV}$  at  $B = 3 \text{ T}$  in (a) and  $B = 15 \text{ T}$  in (b). (c) The landau bands plotted using Eq. (20) with the same parameters and magnetic field as (b). In (a), no Weyl points are formed. In (b) and (c), a pair of Weyl points is generated. (b) and (c) represent two different ways of labeling the two  $n = 0$  bands. Diagram (b) is denoted by the true Lowest Landau index, wherein a band inversion occurs for  $|k_z| < k_w$ . Diagram (c) is denoted by the normal band index  $\xi$ .

#### IV. CALCULATIONS OF CONDUCTIVITIES

The longitudinal and Hall conductivities are calculated by the Kubo-Středa formula [10],

$$\sigma_{ij} = \frac{\hbar}{2\pi V} \int d\omega f(\omega) \text{Tr} \left[ \hat{J}_i \frac{\partial G^R(\omega)}{\partial \omega} \hat{J}_j (G^A(\omega) - G^R(\omega)) - (G^A(\omega) - G^R(\omega)) \hat{J}_j \frac{\partial G^A(\omega)}{\partial \omega} \hat{J}_i \right]. \quad (22)$$

Here,  $V$  stands for the volume,  $f(\omega) = \frac{1}{e^{\beta(\omega - E_F)} + 1}$  represents the Fermi distribution for energy level  $\omega$ , where  $E_F$  represents the Fermi energy and  $\beta = \frac{1}{k_B T}$  with  $T$  being the temperature. The trace denotes summations over Landau level indices  $n, \nu, \mu$  and wave vectors  $\mathbf{k}$ .  $\hat{J}_{i=x,y,z} = \frac{-e\partial H_0(\mathbf{\Pi})}{\hbar\partial \Pi_i}$  denotes the current operator along the  $i$ -direction, and  $G^{R/A}(\omega) = \frac{1}{\omega - H_0(\mathbf{\Pi}) \pm i\Gamma}$  represents the advanced and retarded Green's functions, respectively, with  $\Gamma$  denoting the broadening of the bands. Temporarily, we directly assume the Landau band broadening parameter  $\Gamma$  to be constant, although we will calculate this quantity through disorder scattering [11–14] in Sec. VIII. The specific forms of the electric current operators are given by

$$\begin{aligned} \hat{J}_x &= -\frac{e}{\hbar} \frac{\partial H_0(\mathbf{\Pi})}{\partial \Pi_x} = -\frac{e}{\hbar} (\hbar v_x \tau_z \sigma_x + 2M_x \Pi_x \tau_0 \sigma_z) = -ev_x [\tau_z \sigma_x + \gamma(a + a^\dagger) \tau_0 \sigma_z], \\ \hat{J}_y &= -\frac{e}{\hbar} \frac{\partial H_0(\mathbf{\Pi})}{\partial \Pi_y} = ev_y [\tau_0 \sigma_y + i\gamma(a^\dagger - a) \tau_0 \sigma_z], \end{aligned} \quad (23)$$

where  $\gamma = \frac{\sqrt{2}M_\perp}{\hbar v_\perp \ell_B}$ .

### A. Longitudinal conductivity

The longitudinal conductivity  $\sigma_{xx}$  is calculated by setting  $i = j = x$  in Eq. (22). After performing the calculation of “Tr” in Eq. (22) using the basis of Landau levels  $|n\mathbf{k}, \nu, \mu\rangle$ , the longitudinal conductivity can be written as

$$\sigma_{xx} = \frac{\hbar}{V} \sum_{\mathbf{k}} \sum_{n\nu\mu} \sum_{n'\nu'\mu'} |\langle n\mathbf{k}, \nu, \mu | J_x | n'\mathbf{k}, \nu', \mu' \rangle|^2 \int \frac{d\omega}{4\pi} \frac{\partial f(\omega)}{\partial \omega} (G_{n\nu\mu}^A(\omega) - G_{n\nu\mu}^R(\omega)) (G_{n'\nu'\mu'}^A(\omega) - G_{n'\nu'\mu'}^R(\omega)), \quad (24)$$

where  $G_{n\nu\mu}^{R/A}(\omega, \mathbf{k}) = \frac{1}{\omega - E_{n\nu}^{\mu}(\mathbf{k}) \pm i\Gamma}$  represent the advanced and retarded Green functions for Landau band  $|n\mathbf{k}, \nu, \mu\rangle$ , respectively. For extremely low temperature, we take  $\frac{\partial f(\omega)}{\partial \omega} \approx -\delta(\omega - E_F)$ . After substituting Eq. (23) into Eq. (24), performing the summation for  $n', \nu', \mu'$ , and finishing the integral for  $k_x$  and  $k_y$ ,  $\sigma_{xx}$  is given by

$$\sigma_{xx} = \frac{\hbar v_{\perp}^2 e^2}{2\pi \ell_B^2} \int \frac{dk_z}{2\pi} \sum_{n \geq 0} \sum_{\mu, \nu, \nu' = \pm} \frac{1}{\pi} \frac{\Gamma^2}{[(E_{n\nu}^{\mu} - E_F)^2 + \Gamma^2] [(E_{n+1\nu'}^{\mu} - E_F)^2 + \Gamma^2]} \left( C_{n, \nu, \mu}^{n+1, \nu', \mu} \right)^2, \quad (25)$$

where

$$\begin{aligned} C_{n, \mu, \mu}^{n+1, \mu, \mu} &= \sin \frac{\theta_n}{2} \cos \frac{\theta_{n+1}}{2} + \gamma \sqrt{n} \cos \frac{\theta_n}{2} \cos \frac{\theta_{n+1}}{2} - \gamma \sqrt{n+1} \sin \frac{\theta_n}{2} \sin \frac{\theta_{n+1}}{2}, \\ C_{n, \bar{\mu}, \mu}^{n+1, \mu, \mu} &= \cos \frac{\theta_n}{2} \cos \frac{\theta_{n+1}}{2} - \gamma \sqrt{n} \sin \frac{\theta_n}{2} \cos \frac{\theta_{n+1}}{2} - \gamma \sqrt{n+1} \cos \frac{\theta_n}{2} \sin \frac{\theta_{n+1}}{2}, \\ C_{n, \mu, \bar{\mu}}^{n+1, \bar{\mu}, \mu} &= \sin \frac{\theta_n}{2} \sin \frac{\theta_{n+1}}{2} + \gamma \sqrt{n} \cos \frac{\theta_n}{2} \sin \frac{\theta_{n+1}}{2} + \gamma \sqrt{n+1} \sin \frac{\theta_n}{2} \cos \frac{\theta_{n+1}}{2}, \\ C_{n, \bar{\mu}, \bar{\mu}}^{n+1, \bar{\mu}, \mu} &= \cos \frac{\theta_n}{2} \sin \frac{\theta_{n+1}}{2} - \gamma \sqrt{n} \sin \frac{\theta_n}{2} \sin \frac{\theta_{n+1}}{2} + \gamma \sqrt{n+1} \cos \frac{\theta_n}{2} \cos \frac{\theta_{n+1}}{2}, \end{aligned} \quad (26)$$

with  $\bar{\mu} = -\mu$  and  $\theta_0^{\mu} = 0$ . The sum of  $\mu, \nu, \nu'$  results in eight terms for each  $n$ , and it can be demonstrated that the summation with respect to  $n$  in the above expression is absolutely convergent. In the quantum limit, the term with  $n = 0$  significantly dominates, whereas contributions from terms with  $n \geq 1$  can be safely neglected. As a result, the  $\sigma_{xx}$  can be written as

$$\begin{aligned} \sigma_{xx} \approx \frac{\hbar v_{\perp}^2 e^2}{2\pi^2 \ell_B^2} \int \frac{dk_z}{2\pi} \left\{ \frac{\Gamma^2}{(E_{0+} - E_F)^2 + \Gamma^2} \left[ \frac{(\cos \frac{\theta_1}{2} - \gamma \sin \frac{\theta_1}{2})^2}{(E_{1-} - E_F)^2 + \Gamma^2} + \frac{(\sin \frac{\theta_1}{2} + \gamma \cos \frac{\theta_1}{2})^2}{(E_{1+} - E_F)^2 + \Gamma^2} \right] \right. \\ \left. + \frac{\Gamma^2}{(E_{0-} - E_F)^2 + \Gamma^2} \left[ \frac{(\cos \frac{\theta_1}{2} - \gamma \sin \frac{\theta_1}{2})^2}{(E_{1+} - E_F)^2 + \Gamma^2} + \frac{(\sin \frac{\theta_1}{2} + \gamma \cos \frac{\theta_1}{2})^2}{(E_{1-} - E_F)^2 + \Gamma^2} \right] \right\}. \end{aligned} \quad (27)$$

These four terms correspond to the four virtual scattering processes illustrated in Fig. 2. With Eq. (27),  $\frac{\partial \sigma_{xx}}{\partial E_F}$  can be directly obtained.

### B. Hall conductivity

The Hall conductivity  $\sigma_{xy}$  is calculated by setting  $i = x$  and  $j = y$  in Eq. (22). Following the calculations of  $\sigma_{xx}$ ,  $\sigma_{xy}$  is found to be

$$\begin{aligned} \sigma_{xy} = \frac{\hbar v_{\perp}^2 e^2}{2\pi^2 \ell_B^2} \int \frac{dk_z}{2\pi} \int d\omega \sum_{n \geq 0} \sum_{\mu, \nu, \nu' = \pm} f(\omega) \left\{ \frac{\Gamma [(E_{n+1\nu'}^{\mu} - E_F)^2 - \Gamma^2]}{[(E_{n\nu}^{\mu} - E_F)^2 + \Gamma^2] [(E_{n+1\nu'}^{\mu} - E_F)^2 + \Gamma^2]^2} \right. \\ \left. - (n\nu) \leftrightarrow (n+1\nu') \right\} \left( C_{n, \nu, \mu}^{n+1, \nu', \mu} \right)^2. \end{aligned} \quad (28)$$

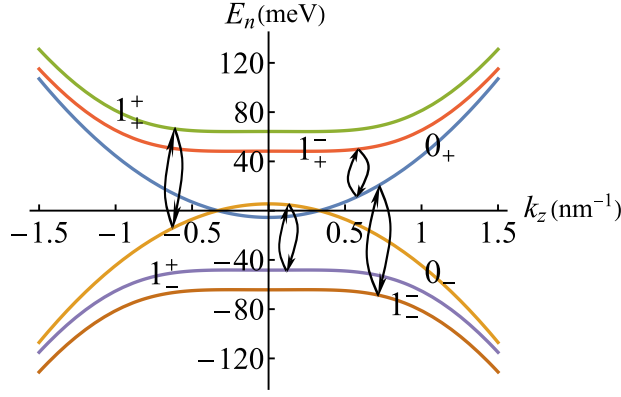

FIG. 2. (a) The four virtual scattering processes between  $n = 0$  and  $n = 1$  Landau Levels contribute most to the longitudinal conductivity. The Landau bands are plotted at  $B = 15$  T with the same parameters as in Fig. 1 except for that  $M_z = 5 \text{ eV} \cdot \text{\AA}^2$ .

In the quantum limit, the term with  $n = 0$  significantly dominates, whereas contributions from terms with  $n \geq 1$  can be safely neglected, Eq. (28) can be further simplified to

$$\begin{aligned} \sigma_{yx} \approx & \frac{\hbar v_{\perp}^2 e^2}{2\pi^2 \ell_B^2} \int \frac{dk_z}{\pi} \int d\omega f(\omega) \left\{ \frac{\Gamma [(E_{1-}^- - \omega)^2 - \Gamma^2] (\cos \frac{\theta_1}{2} - \gamma \sin \frac{\theta_1}{2})^2}{[(E_{0+} - \omega)^2 + \Gamma^2] [(E_{1-}^- - \omega)^2 + \Gamma^2]^2} - \frac{\Gamma [(E_{0+} - \omega)^2 - \Gamma^2] (\cos \frac{\theta_1}{2} - \gamma \sin \frac{\theta_1}{2})^2}{[(E_{0+} - \omega)^2 + \Gamma^2]^2 [(E_{1-}^- - \omega)^2 + \Gamma^2]} \right. \\ & + \frac{\Gamma [(E_{1+}^- - \omega)^2 - \Gamma^2] (\sin \frac{\theta_1}{2} + \gamma \cos \frac{\theta_1}{2})^2}{[(E_{0+} - \omega)^2 + \Gamma^2] [(E_{1+}^- - \omega)^2 + \Gamma^2]^2} - \frac{\Gamma [(E_{0+} - \omega)^2 - \Gamma^2] (\sin \frac{\theta_1}{2} + \gamma \cos \frac{\theta_1}{2})^2}{[(E_{0+} - \omega)^2 + \Gamma^2]^2 [(E_{1+}^- - \omega)^2 + \Gamma^2]} \\ & + \frac{\Gamma [(E_{1-}^+ - \omega)^2 - \Gamma^2] (\sin \frac{\theta_1}{2} + \gamma \cos \frac{\theta_1}{2})^2}{[(E_{0-} - \omega)^2 + \Gamma^2] [(E_{1-}^+ - \omega)^2 + \Gamma^2]^2} - \frac{\Gamma [(E_{0-} - \omega)^2 - \Gamma^2] (\sin \frac{\theta_1}{2} + \gamma \cos \frac{\theta_1}{2})^2}{[(E_{0-} - \omega)^2 + \Gamma^2]^2 [(E_{1-}^+ - \omega)^2 + \Gamma^2]} \\ & \left. + \frac{\Gamma [(E_{1+}^+ - \omega)^2 - \Gamma^2] (\cos \frac{\theta_1}{2} - \gamma \sin \frac{\theta_1}{2})^2}{[(E_{0-} - \omega)^2 + \Gamma^2] [(E_{1+}^+ - \omega)^2 + \Gamma^2]^2} - \frac{\Gamma [(E_{0-} - \omega)^2 - \Gamma^2] (\cos \frac{\theta_1}{2} - \gamma \sin \frac{\theta_1}{2})^2}{[(E_{0-} - \omega)^2 + \Gamma^2]^2 [(E_{1+}^+ - \omega)^2 + \Gamma^2]} \right\}. \end{aligned} \quad (29)$$

The  $\frac{\partial \sigma_{yx}}{\partial E_F}$  is obtained according to Eq. (29), but due to the complexity of the results, the direct expression is not provided here.

## V. FIXING CARRIER DENSITY VS. FIXING FERMI ENERGY

According to the Mott relation [15–17], the thermopower and Nernst coefficient can be obtained from the Hall and longitudinal conductivities by [18]

$$S_{xx} = \frac{\pi^2 k_B^2 T}{3e} \frac{1}{\sigma_{xx}^2 + \sigma_{xy}^2} \left( \sigma_{xx} \frac{\partial \sigma_{xx}}{\partial E_F} + \sigma_{xy} \frac{\partial \sigma_{xy}}{\partial E_F} \right) = \frac{\pi^2 k_B^2 T}{3e} \left( \rho_{xx} \frac{\partial \sigma_{xx}}{\partial E_F} + \rho_{yx} \frac{\partial \sigma_{xy}}{\partial E_F} \right), \quad (30)$$

$$S_{xy} = \frac{\pi^2 k_B^2 T}{3e} \frac{1}{\sigma_{xx}^2 + \sigma_{xy}^2} \left( \sigma_{xx} \frac{\partial \sigma_{xy}}{\partial E_F} - \sigma_{xy} \frac{\partial \sigma_{xx}}{\partial E_F} \right) = \frac{\pi^2 k_B^2 T}{3e} \left( \rho_{xx} \frac{\partial \sigma_{xy}}{\partial E_F} - \rho_{yx} \frac{\partial \sigma_{xx}}{\partial E_F} \right), \quad (31)$$

where the Hall and longitudinal resistivities are given by

$$\rho_{xx} = \frac{\sigma_{xx}}{\sigma_{xx}^2 + \sigma_{xy}^2}, \quad \rho_{yx} = \frac{\sigma_{xy}}{\sigma_{xx}^2 + \sigma_{xy}^2}. \quad (32)$$

Based on Eq. (27) and Eq. (29), we can calculate the values of  $S_{xx}$ ,  $S_{xy}$ ,  $\rho_{xx}$ ,  $\rho_{xy}$ .

To proceed with further calculations, we need to know the dependence of  $E_F$  on  $B$ . Based on previous studies [19, 20], we can treat either the carrier density or the Fermi energy as field-independent. The carrier density in quantum limit is given by

$$n_0 = \frac{1}{2\pi\ell_B^2} \int \frac{dk_z}{2\pi} [f(E_{0+}) - (1 - f(E_{0-}))] = \frac{\sqrt{\pi} \sum_{\mu=\pm} \mu \text{Li}_{1/2} \left( -e^{-\beta(\Delta + M_{\perp}/\ell_B^2 - Z + \mu E_F)} \right)}{4\pi^2 \ell_B^2 \sqrt{\beta M_z}}, \quad (33)$$

where  $\text{Li}_{1/2}(x)$  gives the polylogarithm function of the order 1/2. Eq. (33) provides the constraint relationship among  $n_0$ ,  $E_F$ ,  $B$ . In order to determine how the carrier density and chemical potential change with magnetic field, we are currently lacking an additional theoretical condition. Indeed, this condition has been consistently elusive since the investigation of the quantum Hall effect. Two common approaches are employed to address this issue: firstly, assuming that  $n_0$  remains constant with the magnetic field, enabling an immediate derivation of the behavior of  $E_F$  with respect to  $B$  using Eq. (33); secondly, assuming that  $E_F$  remains constant with  $B$ , allowing us to deduce the behavior of  $n_0$  with respect to  $B$ . These two assumptions have been separately applied in previous theories of strong magnetic field transport [19, 20].

In our work, we have assumed that  $n_0$  is fixed and obtained the  $E_F(B)$  according to Eq. (33). The results are shown in contour plots as Fig. 2(a) and Fig. 3(a) in the main text for weak and strong topological insulators, respectively.

## VI. VALUE OF THE CRITICAL MAGNETIC FIELD FOR THE LIFSHITZ TRANSITION

Before the Lifshitz transition, the carrier density is assumed constant. At the zero-temperature limit, Eq. (33) becomes

$$\begin{aligned} n_0 &= \frac{k_F^+}{2\pi^2 \ell_B^2} \quad \text{before the Lifshitz transition,} \\ &= \frac{k_F^+ - k_F^-}{2\pi^2 \ell_B^2} \quad \text{after the Lifshitz transition.} \end{aligned} \quad (34)$$

where  $k_F^{\pm} = \sqrt{(-\Delta - M_{\perp}/\ell_B^2 + Z \pm E_F)/M_z}$ . Assuming  $n_0$  is constant, the Fermi wave vectors take the form:

$$k_F^+ = 2\pi^2 \ell_B^2 n_0 \quad \text{before the Lifshitz transition,} \quad (35)$$

$$k_F^+ - k_F^- = 2\pi^2 \ell_B^2 n_0 \quad \text{after the Lifshitz transition.} \quad (36)$$

After the Lifshitz transition, the two Fermi wave vectors also satisfy

$$k_F^{+2} + k_F^{-2} = \frac{2[(-M_{\perp}e/\hbar + g\mu_B/2)B - \Delta]}{M_z}. \quad (37)$$

The dependence of  $E_F$  on  $B$  can be found directly after solving for  $k_F^+$  and  $k_F^-$ , and is given by

$$\begin{aligned} E_F &= M_z (2\pi^2 \ell_B^2 n_0)^2 + \Delta + \frac{M_{\perp}}{\ell_B^2} - Z \quad \text{before the Lifshitz transition,} \\ &= \sqrt{M_z (2\pi^2 \ell_B^2 n_0)^2 \left[ Z - M_{\perp}/\ell_B^2 - \Delta - M_z (\pi^2 \ell_B^2 n_0)^2 \right]} \quad \text{after the Lifshitz transition.} \end{aligned} \quad (38)$$

The critical magnetic field for the Lifshitz transition ( $B_2$ ) is determined by  $k_F^- = 0$ , which corresponds to the real root of the equation with respect to  $B$ ,

$$Z - M_{\perp}/\ell_B^2 - \Delta - 2M_z (\pi^2 \ell_B^2 n_0)^2 = 0. \quad (39)$$

## VII. ANALYTICAL VALUE OF THE FLAT NERNST COEFFICIENT

In this section, we analytically demonstrate that the Nernst coefficient remains constant in strong magnetic fields for both weak and strong topological insulators.

### A. Weak topological insulators

Firstly, the Hall and longitudinal conductivities satisfy the relations:

$$\sigma_{xy}(-E_F) = -\sigma_{xy}(E_F), \quad \sigma_{xx}(-E_F) = \sigma_{xx}(E_F), \quad (40)$$

which result in

$$\left. \frac{\partial \sigma_{xx}}{\partial E_F} \right|_{E_F \rightarrow 0} = 0. \quad (41)$$

Therefore, for small values of  $E_F$

$$S_{xy} \approx \frac{\pi^2 k_B^2 T}{3e} \rho_{xx} \frac{\partial \sigma_{xy}}{\partial E_F}. \quad (42)$$

Subsequently, we demonstrated that  $\rho_{xx} \frac{\partial \sigma_{xy}}{\partial E_F}$  converges to a constant by analyzing the asymptotic behaviors of  $\rho_{xx}$  and  $\frac{\partial \sigma_{xy}}{\partial E_F}$  under strong magnetic fields.

We initially concentrate on  $\rho_{xx}$ . At  $E_F = 0$ , Eq. (27) can be expressed as follows:

$$\sigma_{xx} = \frac{2\hbar v_\perp^2 e^2}{2\pi^2 \ell_B^2} \int \frac{dk_z}{2\pi} \left\{ \frac{\Gamma^2}{(E_{0+} - E_F)^2 + \Gamma^2} \left[ \frac{(\cos \frac{\theta_1}{2} - \gamma \sin \frac{\theta_1}{2})^2}{(E_{1-}^- - E_F)^2 + \Gamma^2} + \frac{(\sin \frac{\theta_1}{2} + \gamma \cos \frac{\theta_1}{2})^2}{(E_{1+}^- - E_F)^2 + \Gamma^2} \right] \right\}. \quad (43)$$

For a small value of Landau bands broadening parameter  $\Gamma$ , we can safely make the approximation,

$$\frac{\Gamma}{(E_{0\xi} - E_F)^2 + \Gamma^2} \approx \pi \delta(E_{0\xi} - E_F) \quad (\xi = \pm), \quad (44)$$

Substituting Eq. (44) into Eq. (43) and performing the  $k_z$ -integral yields

$$\sigma_{xx} \approx \frac{\hbar v_\perp^2 e^2}{2\pi^2 \ell_B^2} \frac{\Gamma \Lambda(k_w)}{M_z k_w} \left[ \frac{(\cos \frac{\theta_1}{2} - \gamma \sin \frac{\theta_1}{2})^2}{(E_{1-}^-(k_z))^2} + \frac{(\sin \frac{\theta_1}{2} + \gamma \cos \frac{\theta_1}{2})^2}{(E_{1+}^-(k_z))^2} \right] \Big|_{k_z=k_w}. \quad (45)$$

Noting that the Zeeman splitting  $|Z - M_\perp/\ell_B^2|$  is very small compared to the absolute value of the  $n = 1$  Landau bands at  $k_w$ , we can make further approximations as follows:

$$E_{1\nu}^-(k_z) \approx \nu \sqrt{(M_z k_z^2 + 2M_\perp/\ell_B^2 + \Delta)^2 + (\sqrt{2}\hbar v_\perp/\ell_B)^2}, \quad (46)$$

and then Eq. (45) becomes

$$\begin{aligned} \sigma_{xx} &\approx \frac{\hbar v_\perp^2 e^2}{2\pi^2 \ell_B^2} \frac{\Gamma \Lambda(k_w)}{M_z k_w} \left[ \frac{(\cos \frac{\theta_1}{2} - \gamma \sin \frac{\theta_1}{2})^2 + (\sin \frac{\theta_1}{2} + \gamma \cos \frac{\theta_1}{2})^2}{(M_z k_z^2 + 2M_\perp/\ell_B^2 + \Delta)^2 + (\sqrt{2}\hbar v_\perp/\ell_B)^2} \right] \Big|_{k_z=k_w} \\ &= \frac{\hbar v_\perp^2 e^2}{2\pi^2 \ell_B^2} \frac{\Gamma \Lambda(k_w)}{M_z k_w} \frac{(1 + \gamma^2)}{(Z + M_\perp/\ell_B^2)^2 + (\sqrt{2}\hbar v_\perp/\ell_B)^2} \\ &\approx \frac{\hbar v_\perp^2 e^2}{2\pi^2 \ell_B^2} \frac{\Gamma \Lambda(k_w)}{M_z k_w} \frac{1}{(\sqrt{2}\hbar v_\perp/\ell_B)^2} \\ &= \frac{e^2}{\pi h} \frac{\Gamma}{2M_z k_w}. \end{aligned} \quad (47)$$

Moreover,  $\sigma_{xy} = 0$  when  $E_F = 0$  due to charge neutrality. Therefore, the longitudinal resistivity in strong magnetic fields can be approximated as

$$\rho_{xx} = \frac{1}{\sigma_{xx}} \approx \frac{\pi h}{e^2} \frac{2M_z k_w}{\Gamma}. \quad (48)$$

Now, we consider the asymptotic behaviors of  $\frac{\partial \sigma_{xy}}{\partial E_F}$  under strong magnetic fields. According to Eq. (29),

$$\begin{aligned} \frac{\partial \sigma_{yx}}{\partial E_F} &\approx \frac{\hbar v_{\perp}^2 e^2}{\pi^3 \ell_B^2} \int_0^{+\infty} dk_z \left\{ \frac{\Gamma \left[ (E_{1-}^- - E_F)^2 - \Gamma^2 \right] \left( \cos \frac{\theta_1}{2} - \gamma \sin \frac{\theta_1}{2} \right)^2}{\left[ (E_{0+} - E_F)^2 + \Gamma^2 \right] \left[ (E_{1-}^- - E_F)^2 + \Gamma^2 \right]^2} - \frac{\Gamma \left[ (E_{0+} - E_F)^2 - \Gamma^2 \right] \left( \cos \frac{\theta_1}{2} - \gamma \sin \frac{\theta_1}{2} \right)^2}{\left[ (E_{0+} - E_F)^2 + \Gamma^2 \right]^2 \left[ (E_{1-}^- - E_F)^2 + \Gamma^2 \right]} \right. \\ &\quad + \frac{\Gamma \left[ (E_{1+}^- - E_F)^2 - \Gamma^2 \right] \left( \sin \frac{\theta_1}{2} + \gamma \cos \frac{\theta_1}{2} \right)^2}{\left[ (E_{0+} - E_F)^2 + \Gamma^2 \right] \left[ (E_{1+}^- - E_F)^2 + \Gamma^2 \right]^2} - \frac{\Gamma \left[ (E_{0+} - E_F)^2 - \Gamma^2 \right] \left( \sin \frac{\theta_1}{2} + \gamma \cos \frac{\theta_1}{2} \right)^2}{\left[ (E_{0+} - E_F)^2 + \Gamma^2 \right]^2 \left[ (E_{1+}^- - E_F)^2 + \Gamma^2 \right]} \\ &\quad + \frac{\Gamma \left[ (E_{1-}^+ - E_F)^2 - \Gamma^2 \right] \left( \sin \frac{\theta_1}{2} + \gamma \cos \frac{\theta_1}{2} \right)^2}{\left[ (E_{0-} - E_F)^2 + \Gamma^2 \right] \left[ (E_{1-}^+ - E_F)^2 + \Gamma^2 \right]^2} - \frac{\Gamma \left[ (E_{0-} - E_F)^2 - \Gamma^2 \right] \left( \sin \frac{\theta_1}{2} + \gamma \cos \frac{\theta_1}{2} \right)^2}{\left[ (E_{0-} - E_F)^2 + \Gamma^2 \right]^2 \left[ (E_{1-}^+ - E_F)^2 + \Gamma^2 \right]} \\ &\quad \left. + \frac{\Gamma \left[ (E_{1+}^+ - E_F)^2 - \Gamma^2 \right] \left( \cos \frac{\theta_1}{2} - \gamma \sin \frac{\theta_1}{2} \right)^2}{\left[ (E_{0-} - E_F)^2 + \Gamma^2 \right] \left[ (E_{1+}^+ - E_F)^2 + \Gamma^2 \right]^2} - \frac{\Gamma \left[ (E_{0-} - E_F)^2 - \Gamma^2 \right] \left( \cos \frac{\theta_1}{2} - \gamma \sin \frac{\theta_1}{2} \right)^2}{\left[ (E_{0-} - E_F)^2 + \Gamma^2 \right]^2 \left[ (E_{1+}^+ - E_F)^2 + \Gamma^2 \right]} \right\} \\ &\approx \frac{\hbar v_{\perp}^2 e^2}{\pi^3 \ell_B^2} \frac{1 + \gamma}{(\sqrt{2} \hbar v_{\perp} / \ell_B)^2} \int_0^{+\infty} dk_z \left\{ \frac{2\Gamma^3}{\left[ (E_{0+} - E_F)^2 + \Gamma^2 \right]^2} + \frac{2\Gamma^3}{\left[ (E_{0-} - E_F)^2 + \Gamma^2 \right]^2} \right\} \\ &= \frac{2\sigma_{xx}}{\Gamma} - \Gamma \frac{\partial}{\partial \Gamma} \left( \frac{2\sigma_{xx}}{\Gamma} \right) \end{aligned} \quad (49)$$

$$= \frac{e^2}{\pi \hbar} \frac{1}{M_z k_w}. \quad (50)$$

Substituting Eq. (47) and Eq. (50) into Eq. (42), the flat value of Nernst coefficient is given by,

$$S_{xy}^A = -\frac{\pi^2 k_B^2 T}{3e} \frac{2}{\Gamma}. \quad (51)$$

For non-zero but small values of  $E_F$  (typically for  $E_F \leq 5\text{meV}$ ), the longitudinal conductivity given by Eq. (27) can be approximated as

$$\sigma_{xx} \approx \frac{e^2}{\pi \hbar} \frac{\Gamma}{2} \left( \frac{1}{2M_z k_F^+} + \frac{1}{2M_z k_F^-} \right), \quad (52)$$

and according to Eq. (49),  $\frac{\partial \sigma_{xy}}{\partial E_F}$  is given by

$$\frac{\partial \sigma_{xy}}{\partial E_F} \approx -\frac{e^2}{\pi \hbar} \left( \frac{1}{2M_z k_F^+} + \frac{1}{2M_z k_F^-} \right). \quad (53)$$

By noting that  $k_F^{\pm} = \sqrt{(-\Delta - M_{\perp}/\ell_B^2 + Z \pm E_F)/M_z}$  and  $\Lambda(k_F^{\pm}) \approx 1$ , up to a constant, the Hall conductivity is thus obtained as

$$\sigma_{xy} = -\frac{e^2}{\pi \hbar} (k_F^+ - k_F^-). \quad (54)$$

The charge neutrality point occurs at  $k_F^+ - k_F^-$ , thus the constant is zero, and  $\sigma_{xy}$  is given by Eq. (54).

The Nernst coefficient is simplified to be,

$$S_{xy}^A \approx -\frac{\pi^2 k_B^2 T}{3e} \frac{\frac{\Gamma}{2} \left( \frac{1}{2M_z k_F^+} + \frac{1}{2M_z k_F^-} \right)^2}{\left[ \frac{\Gamma}{2} \left( \frac{1}{2M_z k_F^+} + \frac{1}{2M_z k_F^-} \right) \right]^2 + (k_F^+ - k_F^-)^2}, \quad (55)$$

$$= -\frac{\pi^2 k_B^2 T}{3e} \frac{2\Gamma}{\Gamma^2 + \mathcal{R}^2(M_z, E_F)}, \quad (56)$$

where

$$\mathcal{R}(M_z, E_F) \equiv \frac{4M_z (k_F^+ - k_F^-) k_F^+ k_F^-}{(k_F^+ + k_F^-)} = \frac{4E_F \sqrt{1 - E_F^2/(Z - M_\perp/\ell_B^2 - \Delta)^2}}{1 + \sqrt{1 - E_F^2/(Z - M_\perp/\ell_B^2 - \Delta)^2}}. \quad (57)$$

One can verify that Eq. (56) reduces to Eq. (51) when  $E_F = 0$ . However, for non-zero  $E_F$ , the dependence of  $S_{xy}^A$  on  $B$  is revealed. This can explain why the Nernst plateau disappears when  $n_0$  reaches a certain level, as  $E_F$  becomes relatively large under a strong magnetic field.

### B. Strong topological insulators

For strong topological insulators ( $M_z < M_\perp < 0$ ), the Fermi energy approaches the band bottom of the electronic lowest Landau band. Under strong magnetic fields, the Fermi energy can be approximated as

$$E_F(B) = -M_z \left( \frac{\pi \hbar n}{eB} \right)^2 + Z - M_\perp/\ell_B^2 - \Delta \approx Z - M_\perp/\ell_B^2 - \Delta = (-M_\perp e/\hbar + g\mu_B/2) B - \Delta, \quad (58)$$

which means that  $E_F$  increases linearly with  $B$ . Substituting such  $E_F(B)$  into Eq. (27), the longitudinal conductivity can be approximated as

$$\begin{aligned} \sigma_{xx} &= \frac{\hbar v_\perp^2 e^2}{2\pi^2 \ell_B^2} \int \frac{dk_z}{2\pi} \left\{ \frac{\Gamma^2}{(E_{0+} - E_F)^2 + \Gamma^2} \left[ \frac{(\cos \frac{\theta_1}{2} - \gamma \sin \frac{\theta_1}{2})^2}{(E_{1-}^- - E_F)^2 + \Gamma^2} + \frac{(\sin \frac{\theta_1}{2} + \gamma \cos \frac{\theta_1}{2})^2}{(E_{1+}^- - E_F)^2 + \Gamma^2} \right] \right. \\ &\quad \left. + \frac{\Gamma^2}{(E_{0-} - E_F)^2 + \Gamma^2} \left[ \frac{(\cos \frac{\theta_1}{2} - \gamma \sin \frac{\theta_1}{2})^2}{(E_{1+}^+ - E_F)^2 + \Gamma^2} + \frac{(\sin \frac{\theta_1}{2} + \gamma \cos \frac{\theta_1}{2})^2}{(E_{1-}^+ - E_F)^2 + \Gamma^2} \right] \right\} \\ &\approx \frac{\hbar v_\perp^2 e^2}{2\pi^2 \ell_B^2} \int \frac{dk_z}{2\pi} \left[ \frac{\Gamma^2}{(M_z k_z^2)^2 + \Gamma^2} \frac{1 + \gamma^2}{(\sqrt{2}\hbar v_\perp/\ell_B)^2} + \frac{\Gamma^2}{[M_z k_z^2 + 2(Z - M_\perp/\ell_B^2 - \Delta)]^2 + \Gamma^2} \frac{1 + \gamma^2}{(\sqrt{2}\hbar v_\perp/\ell_B)^2} \right] \\ &\approx \frac{e^2}{\pi \hbar} \frac{\sqrt{\Gamma}}{4\sqrt{2}|M_z|} \left[ 1 + \frac{\sqrt{\Gamma} \sqrt{\Gamma^2 + 4(Z - M_\perp/\ell_B^2 - \Delta)^2 - 2(Z - M_\perp/\ell_B^2 - \Delta)}}{\sqrt{\Gamma^2 + 4(Z - M_\perp/\ell_B^2 - \Delta)^2}} \right] \\ &\approx \frac{e^2}{\pi \hbar} \frac{\sqrt{\Gamma}}{4\sqrt{2}|M_z|}. \end{aligned} \quad (59)$$

Following the above approximation process, we can obtain

$$\begin{aligned} \frac{\partial \sigma_{xx}}{\partial E_F} &\approx \frac{\hbar v_\perp^2 e^2}{2\pi^2 \ell_B^2} \int \frac{dk_z}{2\pi} \left\{ \left[ \frac{\partial}{\partial E_F} \frac{\Gamma^2}{(E_{0+} - E_F)^2 + \Gamma^2} \right] \left[ \frac{(\cos \frac{\theta_1}{2} - \gamma \sin \frac{\theta_1}{2})^2}{(E_{1-}^- - E_F)^2 + \Gamma^2} + \frac{(\sin \frac{\theta_1}{2} + \gamma \cos \frac{\theta_1}{2})^2}{(E_{1+}^- - E_F)^2 + \Gamma^2} \right] \right. \\ &\quad \left. + \left[ \frac{\partial}{\partial E_F} \frac{\Gamma^2}{(E_{0-} - E_F)^2 + \Gamma^2} \right] \left[ \frac{(\cos \frac{\theta_1}{2} - \gamma \sin \frac{\theta_1}{2})^2}{(E_{1+}^+ - E_F)^2 + \Gamma^2} + \frac{(\sin \frac{\theta_1}{2} + \gamma \cos \frac{\theta_1}{2})^2}{(E_{1-}^+ - E_F)^2 + \Gamma^2} \right] \right\} \\ &\approx \frac{\hbar v_\perp^2 e^2}{2\pi^2 \ell_B^2} \int \frac{dk_z}{2\pi} \left[ \frac{2(M_z k_z^2) \Gamma^2}{[(M_z k_z^2)^2 + \Gamma^2]^2} \frac{1 + \gamma^2}{(\sqrt{2}\hbar v_\perp/\ell_B)^2} + \frac{2[M_z k_z^2 + 2(Z - M_\perp/\ell_B^2 - \Delta)] \Gamma^2}{[M_z k_z^2 + 2(Z - M_\perp/\ell_B^2 - \Delta)]^2 + \Gamma^2} \frac{1 + \gamma^2}{(\sqrt{2}\hbar v_\perp/\ell_B)^2} \right] \\ &\approx \frac{e^2}{\pi \hbar} \frac{1}{8\sqrt{2}|M_z| \Gamma}. \end{aligned} \quad (60)$$

The asymptotic behaviors of  $\frac{\partial \sigma_{xy}}{\partial E_F}$  can be derived from Eq. (49), which holds at low temperatures and is valid here.

$$\frac{\partial \sigma_{yx}}{\partial E_F} \approx \frac{e^2}{\pi \hbar} \frac{3}{4\sqrt{2}|M_z| \Gamma}. \quad (61)$$

The Hall conductivity is a constant in a strong magnetic field, which cannot be deduced from Eq. (61) as in the case of weak topological insulators. We need to approximate it according to Eq. (29),

$$\begin{aligned}
\sigma_{yx} &\approx \frac{\hbar v_{\perp}^2 e^2}{2\pi^2 \ell_B^2} \int \frac{dk_z}{\pi} \int d\omega f(\omega) \left\{ \frac{\Gamma}{[(E_{0+} - \omega)^2 + \Gamma^2]} \frac{1 + \gamma^2}{(\sqrt{2}\hbar v_{\perp}/\ell_B)^2} - \frac{\Gamma[(E_{0+} - \omega)^2 - \Gamma^2]}{[(E_{0+} - \omega)^2 + \Gamma^2]^2} \frac{1 + \gamma^2}{(\sqrt{2}\hbar v_{\perp}/\ell_B)^2} \right. \\
&\quad \left. + \frac{\Gamma}{[(E_{0-} - \omega)^2 + \Gamma^2]} \frac{1 + \gamma^2}{(\sqrt{2}\hbar v_{\perp}/\ell_B)^2} - \frac{\Gamma[(E_{0-} - \omega)^2 - \Gamma^2]}{[(E_{0-} - \omega)^2 + \Gamma^2]^2} \frac{1 + \gamma^2}{(\sqrt{2}\hbar v_{\perp}/\ell_B)^2} \right\} \\
&\approx \frac{\hbar v_{\perp}^2 e^2}{2\pi^2 \ell_B^2} \int \frac{dk_z}{\pi} \int d\omega f(\omega) \left\{ \frac{\Gamma}{[(E_{0+} - \omega)^2 + \Gamma^2]} \frac{1}{(\sqrt{2}\hbar v_{\perp}/\ell_B)^2} - \frac{\Gamma[(E_{0+} - \omega)^2 - \Gamma^2]}{[(E_{0+} - \omega)^2 + \Gamma^2]^2} \frac{1}{(\sqrt{2}\hbar v_{\perp}/\ell_B)^2} \right\} \\
&\approx \frac{\hbar v_{\perp}^2 e^2}{\pi^2 \ell_B^2 (\sqrt{2}\hbar v_{\perp}/\ell_B)^2} \int_{-\infty}^0 d\omega' \int_0^{+\infty} \frac{dk_z}{\pi} \frac{2\Gamma^3}{[(M_z k_z^2 + \omega')^2 + \Gamma^2]^2} \\
&= \frac{e^2}{\pi h} \frac{\sqrt{\Gamma}}{2\sqrt{2}|M_z|}
\end{aligned} \tag{62}$$

### VIII. CALCULATION OF THE THE ENERGY BROADENING PARAMETER

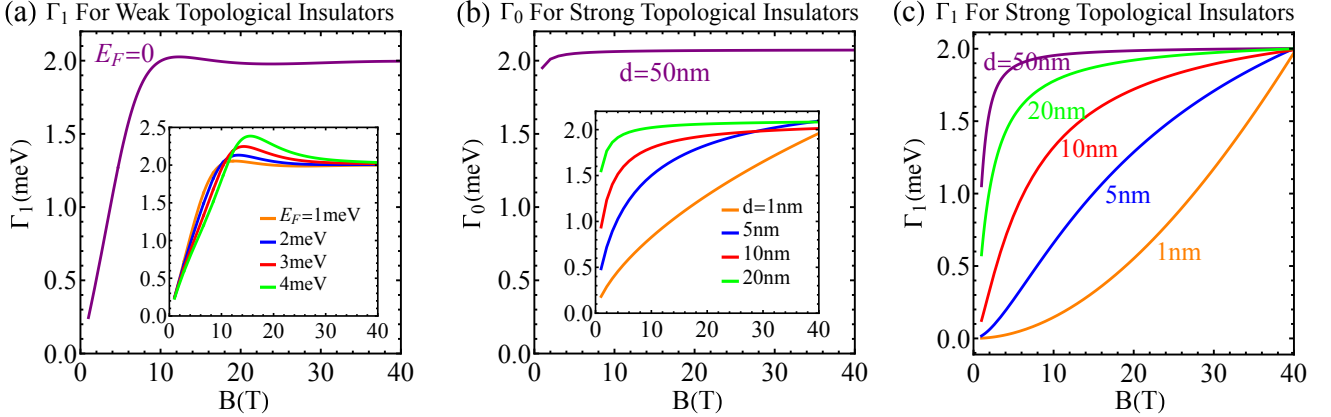

FIG. 3. Dependence of energy broadening parameters on  $B$ . (a) For weak topological insulators, the change of  $\Gamma_1$  with increasing  $B$  for different Fermi energy are plotted according to Eq. (66) with parameters:  $M_{\perp} = -12 \text{ eV} \cdot \text{\AA}^2$ ,  $M_z = 3 \text{ eV} \cdot \text{\AA}^2$ ,  $\Delta = 2.5 \text{ meV}$ ,  $g = 12$ ,  $\Gamma = 2 \text{ meV}$  (The same parameters as in Fig.2 of the main text.),  $n_i u_0^2 = 16 \text{ eV}^2 \cdot \text{nm}^3$ , and  $d = 1.5 \text{ nm}$ . The main diagram plots for  $E_F = 0$ , which represents the ideal 1D Weyl states, while the inset diagram plots for nonzero  $E_F$ . (b), (c) For strong topological insulators, the change of  $\Gamma_0$  and  $\Gamma_1$  with increasing  $B$  for different values of  $d$ , respectively. The parameters are as follows:  $M_z = 12 \text{ eV} \cdot \text{\AA}^2$ ,  $n_0 = 0.8 \times 10^{16} / \text{cm}^3$ , and  $n_i u_0^2 = 12 \text{ eV}^2 \cdot \text{nm}^3$ .

Now we calculate the energy broadening caused by scattering. The results show that for both weak and strong topological insulators, the energy broadenings can be conditionally field-independent.

Given that we are dealing with physics at extremely low temperatures and in the meV energy level, we only consider the scattering from disorder. The disorder scattering potential is assumed to be Gaussian:

$$U(\mathbf{r}) = \sum_i \frac{\sqrt{N_i} u_0}{(d\sqrt{2\pi})^3} e^{-|\mathbf{r} - \mathbf{R}_i|^2 / 2d^2}, \tag{63}$$

where  $N_i$  denotes impurity number and  $u_0$  represents the scattering strength,  $\mathbf{R}_i$  is the impurity position, and  $d$  is the decay length.

The level broadening caused by disorder varies for different Landau bands. In general,  $\Gamma$  should be labeled by the Landau band indices as  $\Gamma_{n\nu\mu}$ . However, for a fixed  $n$ ,  $\Gamma_{n\nu\mu}$  are approximately equal. Since our results depend only

on the  $n = 0$  and  $n = 1$  Landau bands, we denote

$$\Gamma_{0+} \approx \Gamma_{0-} \equiv \Gamma_0; \quad \Gamma_{1++} \approx \Gamma_{1+-} \approx \Gamma_{1-+} \approx \Gamma_{1--} \equiv \Gamma_1. \quad (64)$$

### A. Weak topological insulators

After distinguishing the energy broadening for  $n = 0$  and  $n = 1$  bands, and following the approximations done in Sec. VII A, the value of the Nernst plateau for weak topological insulators takes the form:

$$S_{xy}^A = -\frac{\pi^2 k_B^2 T}{3e} \frac{2}{\Gamma_1}, \quad (65)$$

which means that the energy broadening of  $n = 1$  determines the Nernst plateau. The calculation of  $\Gamma_1 \equiv \hbar/2\tau_1$  directly follows the procedure in the Refs.[12, 14]. The only difference is that there are four  $n = 1$  Landau bands here, whereas there are only two in Refs.[12, 14], but this does not pose any computational difficulties. We present the result directly here,

$$\Gamma_1 = \frac{n_i u_0^2}{16\pi} \frac{\ell_B^2}{(d^2 + \ell_B^2/2)^2} \left[ \frac{(1 + e^{-4(dk_F^+)^2})}{2M_z k_F^+} + \frac{(1 + e^{-4(dk_F^-)^2})}{2M_z k_F^-} \right] \Big|_{k_F^+ = k_w = k_F^-}, \quad (66)$$

where  $n_i = \sum_i N_i/V$  denotes the density of impurity. The detailed calculations can be found in Refs.[12, 14]. This result produces a nearly field-independent  $\Gamma_1$  in the magnetic field range where the Nernst plateau appears. In Fig. 3(a), we plot the variation of  $\Gamma_1$  with  $B$  using the parameters from Fig. 2 in the main text. It can be seen that for an ideal 1D Weyl state ( $E_F = 0$ ),  $\Gamma_1$  is almost field-independent in the strong magnetic field range (the Nernst plateau region). Additionally, as  $E_F$  increases, this field-independent behavior disappears.

### B. Strong topological insulators

Following the approximations done in Sec. VII B, the value of the Nernst plateau for strong topological insulators can be written as,

$$S_{xy}^A = -\frac{\pi^2 k_B^2 T}{3e} \frac{2}{\Gamma_0} \frac{\Gamma_1^2}{16\Gamma_0^2 - 16\Gamma_1\Gamma_0 + 5\Gamma_1^2}. \quad (67)$$

We thus need to calculate  $\Gamma_0 \equiv \hbar/2\tau_0$  and  $\Gamma_1$ . Following the calculations done in Refs.[12, 14], the self-consistent equation within Born approximation for  $\Gamma_0$  takes the form,

$$\Gamma_0 = n_i u_0^2 \int_0^{+\infty} \frac{q_\perp dq_\perp}{2\pi} e^{-q_\perp^2 (d^2 + \ell_B^2/2)} \int_{-\infty}^{+\infty} \frac{dq_z}{2\pi} e^{-q_z^2 d^2} \frac{\Gamma_0}{(E_{0+}(q_z) - E_F)^2 + \Gamma_0^2}. \quad (68)$$

Therefore,  $\Gamma_0$  is determined by the following equation,

$$1 \approx \frac{n_i u_0^2}{\pi (2d^2 + \ell_B^2)} \int_{-\infty}^{+\infty} \frac{dq_z}{2\pi} e^{-q_z^2 d^2} \frac{1}{|M_z|^2 k_z^4 + \Gamma_0^2} \equiv \frac{n_i u_0^2 \mathcal{F}(M_z, d, \Gamma_0)}{\pi (2d^2 + \ell_B^2)}. \quad (69)$$

As  $\mathcal{F}(M_z, d, \Gamma_0)$  is field-independent, when  $d \gg \ell_B$ , a field-independent  $\Gamma_0$  can be obtained by solving  $\mathcal{F}(M_z, d, \Gamma_0) = 2\pi d^2/(n_i u_0^2)$ . In Fig. 3(b), we show the behavior of  $\Gamma_0(B)$ . It can be seen that when  $d = 50\text{nm} (\gg \ell_B \sim 5\text{nm})$ ,  $\Gamma_0(B)$  quickly becomes a constant as  $B$  increased. In the inset, we demonstrate the different behaviors of  $\Gamma_0(B)$  during the transition from  $d < \ell_B$  to  $d \gg \ell_B$ , further indicating that a field-independent  $\Gamma_0(B)$  requires  $d \gg \ell_B$ .

$\Gamma_1$  for strong topological insulators takes a similar form as Eq. (66) but without  $k_F^-$ , which is given by

$$\begin{aligned} \Gamma_1 &= \frac{n_i u_0^2}{16\pi} \frac{\ell_B^2}{(d^2 + \ell_B^2/2)^2} \frac{1 + e^{-4(dk_F^+)^2}}{2M_z k_F^+} \\ &= \frac{n_i u_0^2}{16\pi} \frac{\ell_B^2}{(d^2 + \ell_B^2/2)^2} \frac{1 + e^{-4[d(2\pi^2 \ell_B^2 n_0)]^2}}{2M_z (2\pi^2 \ell_B^2 n_0)}. \end{aligned} \quad (70)$$

For  $d \gg \ell_B$ ,  $\Gamma_1$  can be approximated in the strong magnetic fields as

$$\Gamma_1 \approx \frac{n_i u_0^2}{16\pi} \frac{\ell_B^2}{d^4} \frac{2}{2M_z (2\pi^2 \ell_B^2 n_0)} = \frac{n_i u_0^2}{32\pi^3 M_z n_0 d^4}. \quad (71)$$

The dependence of  $\Gamma_1$  on  $B$  for different values of  $d$  are depicted in Fig. 3(c), which shows that  $\Gamma_1$  is field-independent in strong magnetic field when  $d \gg \ell_B$ .

- 
- [1] S.-Q. Shen, *Topological Insulators*, 2nd ed. (Springer-Verlag, Berlin Heidelberg, 2017).
  - [2] L. Fu, C. L. Kane, and E. J. Mele, “Topological Insulators in Three Dimensions”, *Phys. Rev. Lett.* **98**, 106803 (2007).
  - [3] L. Fu and C. L. Kane, “Topological insulators with inversion symmetry”, *Phys. Rev. B* **76**, 045302 (2007).
  - [4] B. Yan, L. Mchler, and C. Felser, “Prediction of weak topological insulators in layered semiconductors”, *Phys. Rev. Lett.* **109**, 116406 (2012).
  - [5] H. Zhang, C.-X. Liu, X.-L. Qi, X. Dai, Z. Fang, and S.-C. Zhang, “Topological insulators in Bi<sub>2</sub>Se<sub>3</sub>, Bi<sub>2</sub>Te<sub>3</sub> and Sb<sub>2</sub>Te<sub>3</sub> with a single Dirac cone on the surface”, *Nat. Phys.* **5**, 438 (2009).
  - [6] Y. Jiang, J. Wang, T. Zhao, Z. L. Dun, Q. Huang, X. S. Wu, *et al.*, “Unraveling the Topological Phase of ZrTe<sub>5</sub> via Magnetoinfrared Spectroscopy”, *Phys. Rev. Lett.* **125**, 046403 (2020).
  - [7] R. Y. Chen, Z. G. Chen, X.-Y. Song, J. A. Schneeloch, G. D. Gu, F. Wang, and N. L. Wang, “Magnetoinfrared Spectroscopy of Landau Levels and Zeeman Splitting of Three-Dimensional Massless Dirac Fermions in ZrTe<sub>5</sub>”, *Phys. Rev. Lett.* **115**, 176404 (2015).
  - [8] W. Wu, Z. Shi, Y. Du, Y. Wang, F. Qin, X. Meng, *et al.*, “Topological Lifshitz transition and one-dimensional Weyl mode in HfTe<sub>5</sub>”, *Nat. Mater.* **22**, 84 (2023).
  - [9] E. Martino, I. Crassee, G. Eguchi, D. Santos-Cottin, R. D. Zhong, G. D. Gu, *et al.*, “Two-Dimensional Conical Dispersion in ZrTe<sub>5</sub> Evidenced by Optical Spectroscopy”, *Phys. Rev. Lett.* **122**, 217402 (2019).
  - [10] P. Středa, “Theory of quantised hall conductivity in two dimensions”, *J. Phys. C* **15**, L717 (1982).
  - [11] A. A. Abrikosov, “Quantum magnetoresistance”, *Phys. Rev. B* **58**, 2788 (1998).
  - [12] H.-Z. Lu, S.-B. Zhang, and S.-Q. Shen, “High-field magnetoconductivity of topological semimetals with short-range potential”, *Phys. Rev. B* **92**, 045203 (2015).
  - [13] H.-Z. Lu and S.-Q. Shen, “Weak antilocalization and localization in disordered and interacting Weyl semimetals”, *Phys. Rev. B* **92**, 035203 (2015).
  - [14] S.-B. Zhang, H.-Z. Lu, and S.-Q. Shen, “Linear magnetoconductivity in an intrinsic topological Weyl semimetal”, *New J. Phys.* **18**, 053039 (2016).
  - [15] N. Mott and E. Davis, *Electronic Processes in Non-Crystalline Materials* (OUP Oxford, 2012).
  - [16] M. Jonson and G. D. Mahan, “Mott’s formula for the thermopower and the Wiedemann-Franz law”, *Phys. Rev. B* **21**, 4223 (1980).
  - [17] M. Jonson and S. M. Girvin, “Thermoelectric effect in a weakly disordered inversion layer subject to a quantizing magnetic field”, *Phys. Rev. B* **29**, 1939 (1984).
  - [18] J. L. Zhang, C. M. Wang, C. Y. Guo, X. D. Zhu, Y. Zhang, J. Y. Yang, *et al.*, “Anomalous Thermoelectric Effects of ZrTe<sub>5</sub> in and beyond the Quantum Limit”, *Phys. Rev. Lett.* **123**, 196602 (2019).
  - [19] G. D. Mahan, *Many Particle Physics, Third Edition* (Plenum, New York, 2000).
  - [20] C.-L. Zhang, C. M. Wang, Z. Yuan, X. Xu, G. Wang, C.-C. Lee, *et al.*, “Non-saturating quantum magnetization in Weyl semimetal TaAs”, *Nat. Commun.* **10**, 1028 (2019).
